# Supplementary material for: LeRF: Learning Resampling Function for Adaptive and Efficient Image Interpolation
Source: arXiv:2407.09935 source file (2024-07-13)
Supplement: Supplementary file 1 [file abl_suppsize.tex]

% Please add the following required packages to your document preamble:
% \usepackage{multirow}
% \usepackage{graphicx}
% booktabs for table
% https://jdhao.github.io/2019/08/27/latex_table_with_booktabs/

\begin{table}[t]
  \caption{Ablation analysis on the network architeture on the Set5 dataset. ``Ours'' denotes the LUT performance of LeRF, while ``Ours net'' denotes the DNN performance of LeRF. ``Ours net-A'' and ``Ours net-B'' are two variants of LeRF whose DNN have larger receptive field sizes.}
  \centering
  \resizebox{0.9\columnwidth}{!}{%
    \begin{tabular}{lHrr|ccc} \toprule
      & Supp. Size.  & MACs & Supp Size & $\times2$ & $\times3$ & $\times4$ \\ \midrule
      LeRF-G (Ours) & - & 57.69M & $2\times2$ & 35.71 & 32.02 & 30.15 \\
      LeRF-G & 84.36K & ?M & $3\times3$ & 36.11 & 32.23 & 30.28 \\
      LeRF-G & 79.24K & ?M & $\times 44$ & 36.23 & 32.58 & 30.71 \\
      \bottomrule     
    \end{tabular}%
    }
    \label{tab:abl_supp}
    \end{table}
